# Supplementary material for: Optimal Fairness Scheduling for Coded Caching in Multi-AP Multi-antenna WLAN
Source: arXiv:2312.02595 source file (2023-12-06)
Supplement: Supplementary file 1 [file Appendix.tex]

%\subsection{``Random Greedy Association" Algorithm}

\begin{algorithm}
\caption{Random Greedy Association}
\label{alg:main_body}
\begin{algorithmic}[1]
\State $\textsc{Initialize}$
\While{$\min_{k\in [K]} \Sfv(u_k) < v_{\mathrm{limit}}$}
\State $\textsc{Shuffle}(\Bh_{\mathrm{off}})$
\State $\textsc{Shuffle}(\Bd)$
\ForAll{$\hat{d} \in \Bd$}
\State $\textsc{AssignUsers}$
\State $\textsc{AssignHelpers}$
\EndFor
\ForAll{$h_i \in \Bh_{\mathrm{new}}$}
  \State $\Sft(h_i) \gets {1}/{r_{\Sfk(i)}}$
\EndFor
\State $\Bh_{\mathrm{new}} \gets [\;\;]$
\State $t_{\min} \gets \min_{h_i\in{\Bh_{\mathrm{on}}}} \Sft(h_i)$
\ForAll{$h_i\in{\Bh_{\mathrm{on}}}$}
  \State $\Sft(h_i) \gets \Sft(h_i) - t_{\min} $
  \If{$\Sft(h_i)=0$}
   \State Move $h_i$ from $\Bh_{\mathrm{on}}$ to $\Bh_{\mathrm{off}}$
    \ForAll{$l \in [L]$, $\Bm_i[l] \neq 0$}
        %\If{$\Bm_i[l] \neq 0$}
            \State $\Sfv(\Bm_i[l]) \gets \Sfv(\Bm_i[l])+1$  
        %\EndIf
    \EndFor
    \State $\Bm_i \gets [0,0,\cdots,0]$
  \EndIf
\EndFor
\State $T \gets T+t_{\min}$
\EndWhile
\ForAll{$k\in [K]$}
  \State $r_k \gets \Sfv(u_k)/T$
\EndFor
%\State \Return $\Br$
\end{algorithmic}
\end{algorithm}

%\begin{algorithm}
%\caption{Variables Initialize Procedure}
%\label{alg:init}
%\begin{algorithmic}[1]
%\Procedure{Initialize}{}
%    \State $\Bh_{\mathrm{off}} \gets [h_1, h_2, \cdots , h_H]$
%    \State $\Bh_{\mathrm{on}} \gets []$
%    \State $\Bd \gets [d_{\min}, d_{\min}+1, \cdots, d_{\max}]$
%    \State $\Bu_c \gets []$
%\EndProcedure
%\end{algorithmic}
%\end{algorithm}

\begin{algorithm}
\caption{User Assignment Algorithm}
\label{alg:assign_users}
\begin{algorithmic}[1]
\Procedure{AssignUsers}{}

 %\If{$\Bh^{ad}$ is not empty}
  \ForAll{$h_i \in \Bh_{\mathrm{new}}$}
   \ForAll{$k \in [K]$}
    \If{$\Sfd(u_k)=\hat{d}$, $\textsc{Connect}(h_i,u_k) = 1$}
    %$\Bh^{ad}_i\Bu_k\in{\CE_t}$ and $\nexists{}h\in{\CH_{a}},h\neq{\Bh^{ad}_i}$ s.t. $h\Bu_k\in{\CE}$
     \State Add $u_k$ to $\Bu_{\mathrm{cnd}}$ %$\Bu^{ct} \gets [\Bu^{ct},\Bu_k]$
    \EndIf
   \EndFor
   \State $\textsc{Shuffle}(\Bu_{\mathrm{cnd}})$
   \ForAll{$u_k \in \Bu_{\mathrm{cnd}}$}
     \If{$\Bm_i[\SfL(u_k)] = 0$}
     %\If{$l:=c(\Bu^{ct}_k)$th row of $\Bv(\Bh_{\mathrm{off}}^{ad})$ is empty}
       %\State $\Bv_{l}(\Bh_{\mathrm{off}}^{ad}) \gets \Bu^{ct}_k$
       \State $\Bm_i[\SfL(u_k)] \gets u_k$
     \EndIf
   \EndFor
   \State $\Bu_{\mathrm{cnd}} \gets [\;\;]$  
  \EndFor
% \EndIf
\EndProcedure
\end{algorithmic}
\end{algorithm}

\begin{algorithm}
\caption{Helper assignment algorithm}
\label{alg:assign_helpers}
\begin{algorithmic}[1]
\Procedure{AssignHelpers}{}
 \ForAll{$h_i \in \Bh_{\mathrm{off}}$}
  \If{$\nexists{u_k}\in{[\Bm_{(i)}]}$ s.t. $ |\Sfx(h_i)-\Sfx(u_k)| \le r_{\mathrm{inter}}$}
   \ForAll{$k \in [K]$}
    \If{$\Sfd(u_k) = \hat{d}$, $\textsc{Connect}(h_i,u_k) = 1$}
     \State Add $u_k$ to $\Bu_{\mathrm{cnd}}$    
    \EndIf
   \EndFor
   \State $\textsc{Shuffle}(\Bu_{\mathrm{cnd}})$ %$\Bu^{ct} \gets g(\Bu^{ct})$
   \ForAll{$u_k \in \Bu_{\mathrm{cnd}}$}
     \If{$\Bm_i[\SfL(u_k)] = 0$}
       \State $\Bm_i[\SfL(u_k)] \gets u_k$
     \EndIf
   \EndFor
    \State $\Bu_{\mathrm{cnd}} \gets [\;\;]$   
  \EndIf
  \If{$\Bm_i$ is not empty}
   \State Remove $h_i$ from $\Bh_{\mathrm{off}}$ and add it to $\Bh_{\mathrm{on}}$, $\Bh_{\mathrm{new}}$
   %\State Remove $\Bh_{\mathrm{off}}[i]$ from $\Bh_{\mathrm{off}}$
  \EndIf
 \EndFor
 \EndProcedure
\end{algorithmic}
\end{algorithm}

\begin{exmp}
\label{exmp:stalling}
Assume that we have $2$ helpers $h_1$ and $h_2$ and we have three users $u_1$, $u_2$, and $u_3$ where $\SfL(u_1)=\SfL(u_2)=\SfL(u_3)=l$. Let $\Sfd(u_1)=\Sfd(u_2)=1$, and $\Sfd(u_3)=2$ such that $|\Sfx(h_1)-\Sfx(u_k)| \le r_{\mathrm{trans}}$ for $k\in{}\lbrace1,3\rbrace$ and $|\Sfx(h_2)-\Sfx(u_k)| \le r_{\mathrm{trans}}$ for $k\in{}\lbrace2,3\rbrace$. Assume we shuffle the helpers but not the degrees, hence $\Bd$ is fixed. 

Let $\Bd=[1,2]$, and so, in the first step, we select $\Bd[1]=1$. 
In the beginning, both helpers are inactive, and so we can start from $h_1$ or $h_2$ depending on the shuffle. Let us start from $h_1$. Since all the helpers are inactive, we directly go to line $5$ of the helper assignment algorithm. There is only one user, i.e., $u_1$, that satisfies line~5 of this algorithm. So, $u_1$ is assigned to $h_1$. Similarly, user $u_2$ is assigned to $h_2$. 
Now, for $\Bd[2]=2 $, user $u_3$ can not be assigned to any of the helpers since they are both interfering with $u_3$, i.e., $\textsc{Connect}(h_k,u_3)=0$ for $h_1$ and $h_2$. 

After $u_1$ and $u_2$ are served, $h_1$ and $h_2$ both become inactive, and we are back to the initial condition and $u_3$ and can not be served. It can be easily verified that a similar issue persists if we set $\Bd=[2,1]$. In this case $u_1$ and $u_2$ can not be served.
%
%Now let $\Bd=[2 1]$ fixed. At first $\textbf{d}[1]=2$. As before, let's start from $h_1$ and we can assign $u_3$ to $h_1$. We cant activate $h_2$ since it is interfering with $u_3$ ,i.e. line $3$ of the helper assignment algorithm. Then we have $\textbf{d}[2]=1$. We can't assign $u_1$ to $h_1$ since $L(u_1)=L(u_3)$ , i.e. line $8$ of the user assignment algorithm. After $u_3$ is served we are back to the initial condition and if we start from $h_2$ because of symmetry again only $u_3$ will be served and $u_1$ and $u_2$ can not be served.
%
%So in this case we need to shuffle also \textbf{d} which corresponds to being able to combine the procedures in the previous paragraphs so that every user $u_k$ can be served.
\end{exmp}
